# Supplementary material for: Anisotropic spin-density distribution and magnetic anisotropy of strained La$_{1-x}$Sr$_x$MnO$_3$ thin films: Angle-dependent x-ray magnetic circular dichroism
Source: arXiv:1706.05183 ancillary file (2018-01-31)
Supplement: Supplementary file 1 [file supfinal.pdf]

## Supplementary Figures

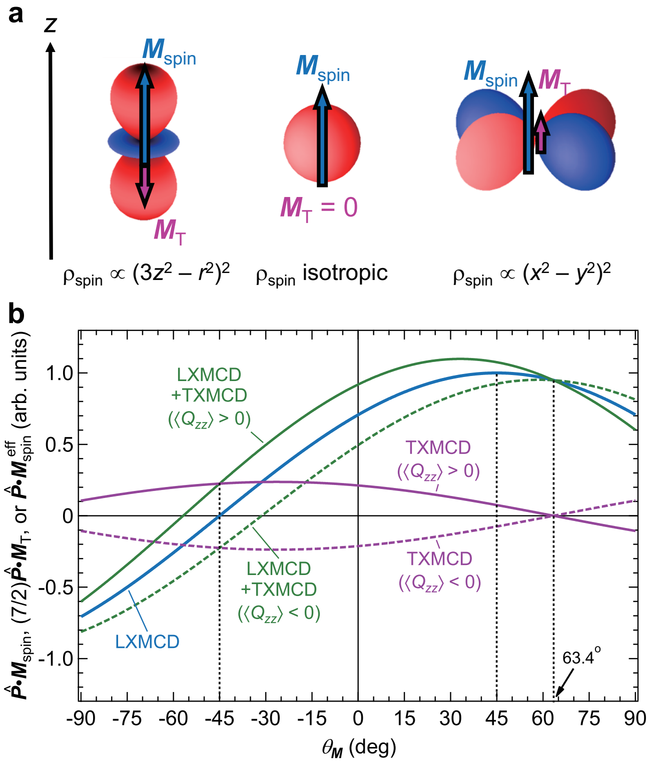


**Supplementary Figure 1**. **Angular dependencies of the spin magnetic moment ($\boldsymbol{M}_{spin}$) and the magnetic dipole term ($\boldsymbol{M}_T$).** (**a**) Relationship between the direction of $\boldsymbol{M}_T$ relative to $\boldsymbol{M}_{spin}$ and the anisotropy of the spin-density distribution ($\rho_{spin}$). For $(3z^2 - r^2)^2$-like $\rho_{spin}$, $\boldsymbol{M}_T$ becomes antiparallel to $\boldsymbol{M}_{spin}$. For $(x^2 - y^2)^2$-like $\rho_{spin}$, $\boldsymbol{M}_T$ becomes parallel to $\boldsymbol{M}_{spin}$. (Here, $\boldsymbol{M}_{spin}$ is along the $z$ direction.) (**b**) Calculated magnetization-angle ($\theta_{\boldsymbol{M}}$) dependencies of $\hat{\boldsymbol{P}}\cdot\boldsymbol{M}_{spin}$, $(7/2)\hat{\boldsymbol{P}}\cdot\boldsymbol{M}_T$, and $\hat{\boldsymbol{P}}\cdot\boldsymbol{M}^{eff}_{spin} = \hat{\boldsymbol{P}}\cdot[\boldsymbol{M}_{spin} + (7/2)\boldsymbol{M}_T]$ for the x-ray incident angle ($\theta_{inc}$) of 45°, where $\hat{\boldsymbol{P}}$ is the unit vector along the light axis (see Fig. 1b in the main text for the deinitions). The first two terms are respectively referred to as the longitudinal x-ray magnetic circular dichroism (LXMCD) and transverse x-ray magnetic circular dichroism (TXMCD) components in the present paper. For $(7/2)\hat{\boldsymbol{P}}\cdot\boldsymbol{M}_T$ and $\hat{\boldsymbol{P}}\cdot\boldsymbol{M}^{eff}_{spin}$, the solid and dashed curves, respectively, describe the cases where the $zz$-component of the electric quadrupole moment tensor ($\langle Q_{zz}\rangle$) is positive and negative, i.e. the electron orbital is $d_{x^2-y^2}$-like and $d_{3z^2-r^2}$-like. The magnitudes of $\boldsymbol{M}_{spin}$ and $\langle Q_{zz}\rangle$ are assumed to be $M_{spin} = 1$ and $(7/2)\langle Q_{zz}\rangle = 0.3$ here.

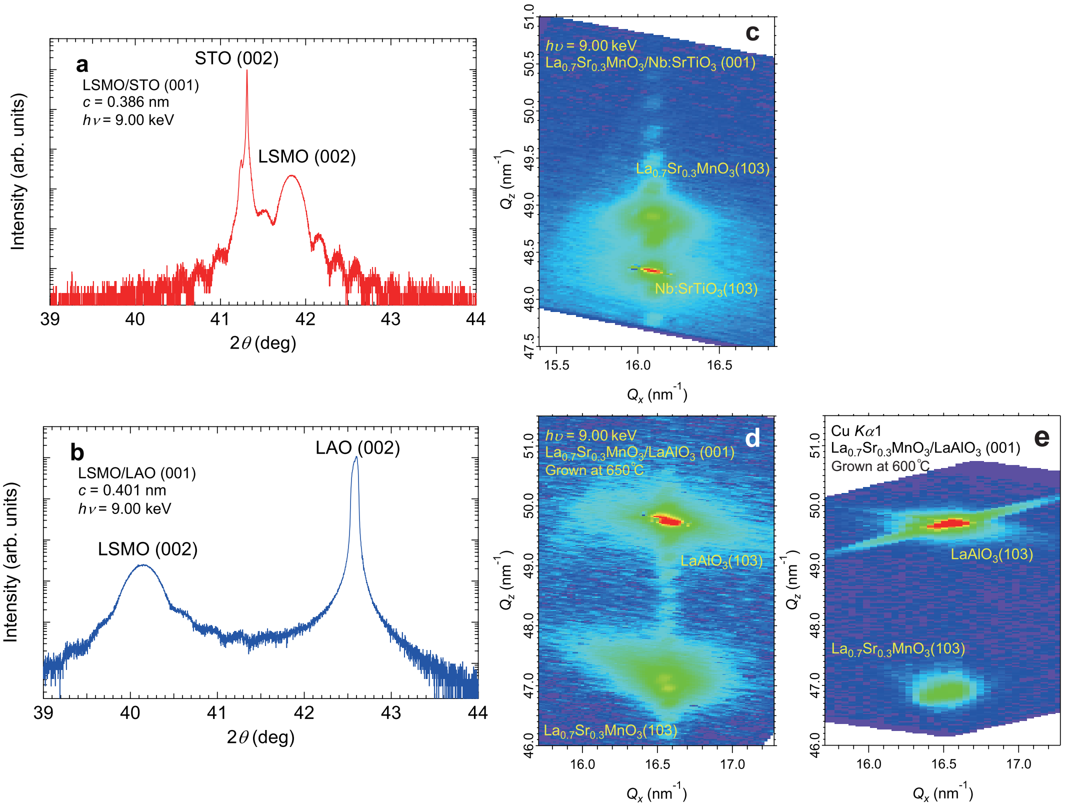


**Supplementary Figure 2**. **X-ray diffraction (XRD) patterns.** (**a, b**) $\theta$-$2\theta$ XRD patterns for the studied $La_{1-x}Sr_xMnO_3$ (LSMO, $x = 0.3$)/Nb-doped $SrTiO_3$ (STO) (**a**) and LSMO ($x = 0.3$)/$LaAlO_3$ (LAO) (**b**) thin films. The out-of-plane lattice constant ($c$) has been estimated to be 0.386 nm and 0.401 nm for the STO and LAO substrates, respectively. (**c-e**) Reciprocal space mapping around the (103) diffraction peak for the LSMO/STO film (**c**), LSMO/LAO film grown at 650 °C (**d**), and LSMO/LAO film grown at 600 °C (**e**). The lattice constants $a$ and $c$ are given by $a = 2\pi/Q_x$ and $c = 3 \times 2\pi/Q_z$.

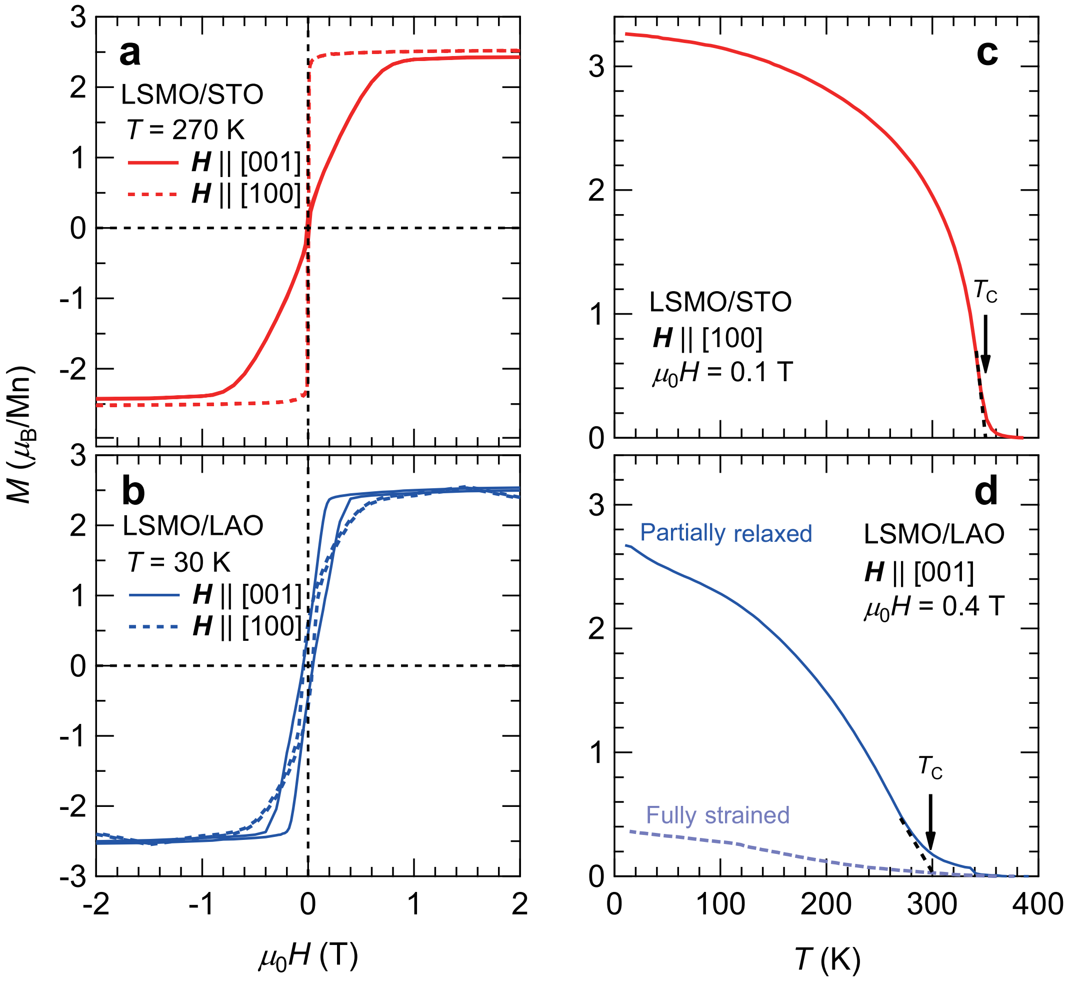


**Supplementary Figure 3**. **Magnetization data measured by superconducting quantum interference device (SQUID) magnetometry.** (**a, b**) Magnetization ($M$)-magnetic-field ($H$) curves of the LSMO/STO (**a**) and LSMO/LAO (**b**) thin films. (**c, d**) Temperature ($T$) dependencies of $M$ for the LSMO/STO (**c**) and LSMO/LAO (**d**) thin films. For the LSMO/LAO films, the $M$-$T$ curves for both the fully strained film (grown at 600 °C) and the partially relaxed film (grown at 650 °C) are shown.

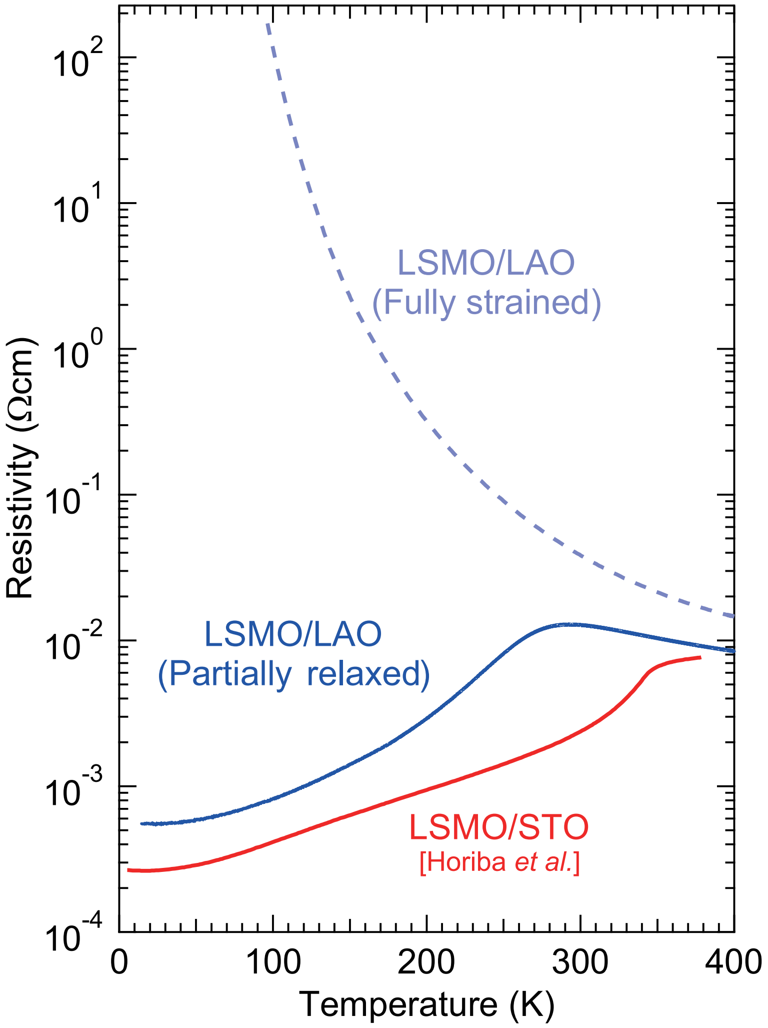


**Supplementary Figure 4. Temperature dependence of the resistivity for the LSMO/STO and LSMO/LAO thin films.** For the LSMO/LAO films, the data for both the fully strained film (grown at 600 °C) and the partially relaxed film (grown at 650 °C) are shown. Since the resistivity measurements are not feasible for the LSMO/STO film due to the conductive Nb-doped STO substrate, we show here the resistivity data for another LSMO thin film grown on a non-doped STO substrate, which was grown essentially under the same conditions as the film studied by XMCD [1].

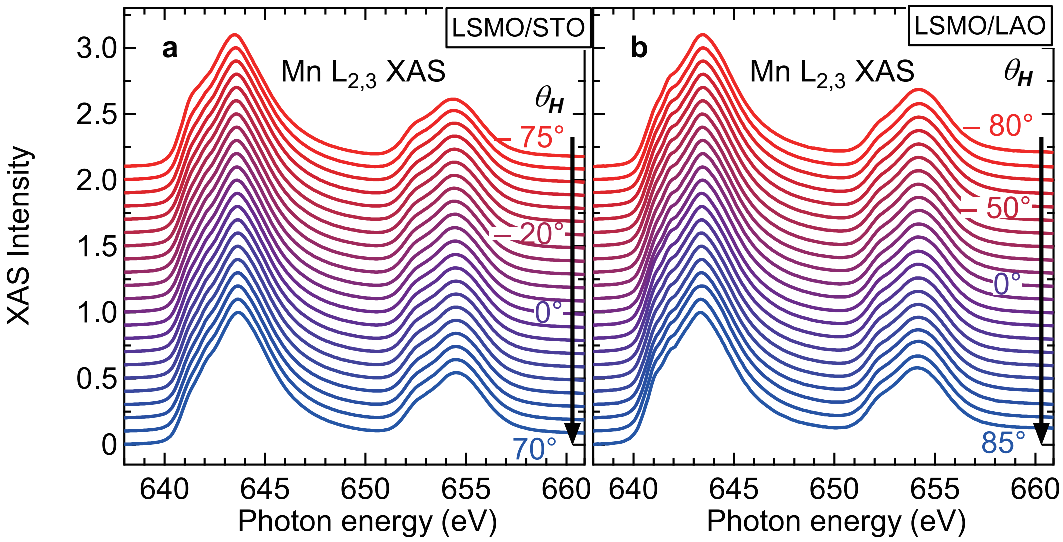


**Supplementary Figure 5. X-ray absorption spectroscopy (XAS) spectra with varying magnetic-field angle ($\theta_H$).** Mn $L_{2,3}$-edge XAS spectra of the LSMO thin films grown on the (**a**) STO and (**b**) LAO substrates with varying $\theta_H$. The XAS spectra are averaged over the positive and negative helicity photons. It can be seen that the spectral line shape of the averaged XAS spectra is almost independent of $\theta_H$.

## Supplementary Tables

**Supplementary Table 1. Simulation parameters used for the cluster-model calculations (in eV).** The $D_{4h}$ symmetry has been assumed. $U_{dd}$: $3d$-$3d$ Coulomb interaction, $U_{pd}$: $2p$-$3d$ Coulomb interaction, $\Delta$: Charge-transfer energy, $(pd\sigma)$: Slater-Koster parameter, $10Dq$: Crystal-field splitting between the $e_g$ and $t_{2g}$ levels, $8Cp$: Crystal-field splitting between the $x^2 - y^2$ and $3z^2 - r^2$ levels ($Cp > 0$ corresponds to the case where the $x^2 - y^2$ level has lower energy than the $3z^2 - r^2$ level) [2].

| $U_{dd}$ | $U_{pd}$ | $\Delta$ | $(pd\sigma)$ | $10Dq$ | $\|8Cp\|$ |
|---|---|---|---|---|---|
| 7.0 | 8.5 | 4.0 | 2.0 | 1.5 | 0.08 |

## Supplementary Notes

### Supplementary Note 1: Principles of angle-dependent x-ray magnetic circular dichroism (XMCD) and transverse XMCD

In this Supplementary Note, we summarize the basic principles of angle-dependent x-ray magnetic circular dichroism (XMCD) and transverse XMCD (TXMCD) [3–6], and the definition and the interpretation of the magnetic dipole term $\boldsymbol{M}_{\mathrm{T}}$.

According to the XMCD orbital [7] and spin [8] sum rules, the orbital ($\boldsymbol{M}_{\mathrm{orb}}$) and spin magnetic moment ($\boldsymbol{M}_{\mathrm{spin}}$) projected along the light axis may be calculated from the integrals of the XMCD spectra ($\Delta I \equiv I^{+} - I^{-}$) and the x-ray absorption spectroscopy (XAS) spectra summed over both helicities ($I \equiv I^{+} + I^{-}$). Here, $I^{+}$ and $I^{-}$ are the XAS intensities as functions of photon energy for the positive and negative helicities, respectively. In the case of $L_{2,3}$ ($2p \to 3d$) absorption edges, the explicit forms of the sum rules are given as follows:

$$\hat{\boldsymbol{P}} \cdot \boldsymbol{M}_{\mathrm{orb}} = -\frac{4}{3}\frac{\Delta I_3 + \Delta I_2}{I_3 + I_2} n_h \mu_B, \tag{1}$$

$$\hat{\boldsymbol{P}} \cdot \boldsymbol{M}_{\mathrm{spin}} + \frac{7}{2}\hat{\boldsymbol{P}} \cdot \boldsymbol{M}_{\mathrm{T}} = -\frac{\Delta I_3 - 2\Delta I_2}{I_3 + I_2} n_h g \mu_B, \tag{2}$$

where $\hat{\boldsymbol{P}}$ is the unit vector along the light axis (see Fig. 1b in the main text for the deinition), subscripts 3 and 2 denote the integrals over the $L_3$ ($2p_{3/2} \to 3d$) and $L_2$ ($2p_{1/2} \to 3d$) absorption edges, respectively, $g$ ($\simeq 2$) denotes the $g$-factor, and $n_h$ denotes the number of holes per atom in the $3d$ level. In Supplementary Eq. (2), $\boldsymbol{M}_{\mathrm{T}}$ is the magnetic dipole term defined using the magnetic dipole operator $\boldsymbol{T}$ as $\boldsymbol{M}_{\mathrm{T}} \equiv -g\mu_B \langle \boldsymbol{T} \rangle$, where

$$\boldsymbol{T} \equiv \boldsymbol{S} - 3(\boldsymbol{S} \cdot \hat{\boldsymbol{r}})\hat{\boldsymbol{r}}. \tag{3}$$

Here, $\hbar\boldsymbol{S}$ is the spin angular momentum operator ($\boldsymbol{M}_{\mathrm{spin}} = -g\mu_B\langle \boldsymbol{S} \rangle$), and $\hat{\boldsymbol{r}}$ is a unit-vector operator defined as $\hat{\boldsymbol{r}} \equiv \boldsymbol{r}/|\boldsymbol{r}|$, using the electron position operator $\boldsymbol{r}$.

$\boldsymbol{M}_{\mathrm{T}}$ represents the spin-density distribution anisotropy [3, 4] as explained below. Here we introduce the electric quadrupole-moment tensor operator $Q_{ij}$ [3, 4] defined by

$$Q_{ij} \equiv \delta_{ij} - 3\hat{r}_i\hat{r}_j \qquad (i, j = x, y, z). \tag{4}$$

The expectation values of $Q_{ij}$'s represent the anisotropy of charge distribution, e.g., it can be shown by direct calculations that $\langle Q_{zz} \rangle = \langle 1 - 3\hat{z}^2 \rangle < 0$ for the $d_{3z^2-r^2}$ orbital while

$\langle Q_{zz}\rangle > 0$ for the $d_{x^2-y^2}$ orbital. Using $Q_{ij}$'s, Supplementary Eq. (3) can be rewritten as $T_i = \sum_j Q_{ij} S_j$. In the limiting case of weak spin-orbit coupling as in $3d$ transition metals, the wave function of the electron may be written as a product of spatial and spin parts, therefore $\langle Q_{ij} S_j\rangle$ can be replaced by $\langle Q_{ij}\rangle\langle S_j\rangle$. Thus one obtains

$$M_{\mathrm{T}}^i = \sum_j \langle Q_{ij}\rangle M_{\mathrm{spin}}^j. \tag{5}$$

Supplementary Eq. (5) shows that $\boldsymbol{M}_{\mathrm{T}}$ is a quantity which is coupled to both the anisotropic charge distribution and the spin magnetic moment. Especially, when the crystal symmetry is higher than $D_{2h}$, $\langle Q_{ij}\rangle$ can be diagonalized if the $x$, $y$, and $z$-axes are chosen parallel to the crystal axes [3], thus

$$M_{\mathrm{T}}^i = \langle Q_{ii}\rangle M_{\mathrm{spin}}^i. \tag{6}$$

Supplementary Eq. (6) shows that $M_{\mathrm{T}}^i$'s ($i = x, y, z$) represent the anisotropy of the spin density along the $i$-axis, since the sign of $M_{\mathrm{T}}^i$ changes whether the spin density is high or low along the $i$-axis [Supplementary Fig. 1a]. We emphasize that these $M_{\mathrm{T}}^i$'s are different from $\langle Q_{ij}\rangle$'s deduced from x-ray linear dichroism (XLD), which are sensitive to the orbital polarization of *all* the electrons regardless of their spin states.

The $\hat{\boldsymbol{P}}\cdot\boldsymbol{M}_{\mathrm{T}}$ term in Supplementary Eq. (2) can be extracted by aligning the spin magnetic moment perpendicular to the incident x rays so that $\hat{\boldsymbol{P}}\cdot\boldsymbol{M}_{\mathrm{spin}} = 0$, i.e., in the so-called TXMCD geometry [4]. In conventional XMCD geometry, i.e., in the longitudinal XMCD (LXMCD) geometry, on the other hand, $\boldsymbol{H}$ is applied parallel to the x rays and the $\hat{\boldsymbol{P}}\cdot\boldsymbol{M}_{\mathrm{spin}}$ term is predominant. Hereafter, we refer to the $(7/2)\hat{\boldsymbol{P}}\cdot\boldsymbol{M}_{\mathrm{T}}$ and $\hat{\boldsymbol{P}}\cdot\boldsymbol{M}_{\mathrm{spin}}$ terms deduced using the spin sum rule as the TXMCD and LXMCD components, respectively. The TXMCD and LXMCD terms show different angular dependencies as functions of $\theta_{\boldsymbol{M}}$ and $\theta_{\mathrm{inc}}$, since the TXMCD component depends not only on the spin state but also on the orbital state of the spin-polarized electrons. In the present case of thin films with uniaxial strain, the angular dependencies of the LXMCD and TXMCD components can be calculated as

$$\begin{aligned} &\hat{\boldsymbol{P}}\cdot\boldsymbol{M}_{\mathrm{spin}} + (7/2)\hat{\boldsymbol{P}}\cdot\boldsymbol{M}_{\mathrm{T}} \\ &\simeq \sum_i \hat{P}_i M_{\mathrm{spin}}^i + (7/2)\sum_i \hat{P}_i\langle Q_{ii}\rangle M_{\mathrm{spin}}^i \\ &= M_{\mathrm{spin}}\cos(\theta_{\boldsymbol{M}} - \theta_{\mathrm{inc}}) + (7/4)\langle Q_{zz}\rangle M_{\mathrm{spin}}(2\cos\theta_{\boldsymbol{M}}\cos\theta_{\mathrm{inc}} - \sin\theta_{\boldsymbol{M}}\sin\theta_{\mathrm{inc}}). \end{aligned} \tag{7}$$

Here, the in-plane rotational symmetry ($\langle Q_{xx}\rangle = \langle Q_{yy}\rangle$) and the traceless property of $\langle Q_{ij}\rangle$ ($2\langle Q_{xx}\rangle + \langle Q_{zz}\rangle = 0$) have been used. In the present study, $\theta_{\rm inc}$ was fixed to 45° and $\theta_{\boldsymbol{M}}$ was varied through varying $\theta_{\boldsymbol{H}}$. The $\theta_{\boldsymbol{M}}$-dependencies of the LXMCD component, TXMCD component, and the sum of them are schematically drawn in Supplementary Fig. 1(b) for $\langle Q_{zz}\rangle > 0$ ($d_{x^2-y^2}$-like) and $\langle Q_{zz}\rangle < 0$ ($d_{3z^2-r^2}$-like). Since the LXMCD and TXMCD components show different $\theta_{\boldsymbol{M}}$-dependencies, it is possible to separate them from the $\theta_{\boldsymbol{M}}$-dependent XMCD spectra. By extracting the TXMCD component from the LXMCD component deduced using the spin sum rule, one can obtain information about the orbital polarization ($\langle Q_{zz}\rangle$) of the *spin-polarized* electrons, namely, the anisotropy of the spin-density distribution.

**Supplementary Note 2: Sample characterization**

Since the purpose of the present study is to reveal the anisotropic spin-density distribution induced by the epitaxial strain, it is necessary to prepare $La_{1-x}Sr_xMnO_3$ (LSMO) films with epitaxial strain. However, a fully strained LSMO ($x = 0.3$) film deposited on a $LaAlO_3$ (LAO) substrate is known to be an antiferromagnetic insulator [9], which is unfavorable for XMCD studies. Here we show the results of sample characterization by x-ray diffraction (XRD), magnetization, and transport measurements in order to ensure that the films measured in the present XMCD study are well strained and at the same time are in the ferromagnetic metallic phase.

Supplementary Figs. 2a and 2b show the $\theta$-$2\theta$ XRD patterns using synchrotron x-ray source for the studied LSMO/STO and LSMO/LAO thin films, respectively. The sharp peaks located at $2\theta = 41.31°$ in Supplementary Fig. 2a and $2\theta = 42.60°$ in Supplementary Fig. 2b are the diffraction peaks from the substrate, while the broader peaks at $2\theta = 41.83°$ in Supplementary Fig. 2a and $2\theta = 40.14°$ in Supplementary Fig. 2b correspond to signals from the LSMO films. The out-of-plane lattice constant of LSMO (in the pseudo-cubic notation) has been estimated to be 0.386 nm (0.401 nm) for the STO (LAO) substrate, and is shorter (longer) than that of the bulk (0.389 nm). This confirms that tensile (compressive) epitaxial strain is applied to the film from the STO (LAO) substrate. In addition, the clear oscillation fringes around the main diffraction peak suggest the sharpness of the surface and the interface between the LSMO film and the substrate.

Supplementary Figs. 2c and 2d respectively show the reciprocal space maps (RMSs) around the LSMO (103) diffraction peak for the LSMO/STO (grown at 1050 °C) and LSMO/LAO (grown at 650 °C) thin films, which are the samples measured in the present XMCD study. In Supplementary Figs. 2e, the RSM for the LSMO/LAO thin film grown at a lower temperature (600 °C) is also shown as a reference. The RSM for LSMO/STO (Supplementary Fig. 2c) exhibits a sharp diffraction peak located at the same $Q_x$ as that of the STO substrate, indicating that the film is almost fully locked to the substrate. On the other hand, as shown in Supplementary Fig. 2d, the diffraction spot for the LSMO/LAO film grown at 650 °C is split into two peaks and has longer tails towards the low-$Q_x$ and high-$Q_z$ sides. This is in contrast to the LSMO/LAO film grown at a lower temperature (600 °C, Supplementary Fig. 2e), which exhibits a sharp diffraction peak and is shown to be fully strained. This indicates that the strain is partially relaxed in the LSMO/LAO film measured in the present XMCD study. Since the fully strained LSMO/LAO film tends to be an antiferromagnetic insulator as shown below and in Ref. 9, we have adopted the partially relaxed film for the XMCD measurement. We also note that the LSMO/LAO film tends to be fully relaxed if the growth temperature is further increased [9].

Supplementary Figures 3a and 3b shows the magnetization curves of the LSMO/STO and the partially relaxed LSMO/LAO thin films, respectively. These magnetization curves show that the magnetic easy axes lie in the plane for the LSMO/STO film and that the easy axis is out-of-plane for the LSMO/LAO film, consistent with previous studies [10, 11]. The temperature dependence of the magnetization for the LSMO/STO and LSMO/LAO thin films are shown in Supplementary Fig. 3c and 3d, respectively. For LSMO/LAO, the data for both the partially relaxed and fully strained films are shown (see Supplementary Figs. 2d and 2e). The partially relaxed LSMO/LAO film exhibits a relatively large saturation magnetization ($\sim 2.5\ \mu_B$/Mn), indicating that the majority part of the film is in the ferromagnetic phase, while the ferromagnetism is almost suppressed in the fully strained film. The Curie temperature ($T_{\mathrm{C}}$) is estimated to be $350 \pm 5$ K for the STO substrate and $300 \pm 10$ K for the LAO substrate.

We note that the difference in the saturation magnetization measured by the SQUID (Supplementary Fig. 3) and XMCD (Table I in the main text) may be explained by the magnetic dead layer near the film surface [12] and the finite the probing depth of XMCD [13]. Assuming that the thickness of the magnetic dead layer ($d$) is 1.6 nm (4 unit cells [12])

and that the probing depth ($\lambda$) is 3 nm, the average magnetic moment detected by XMCD ($M_{\rm av}$) is calculated to be

$$\begin{aligned} M_{\rm av} &= \int_d^{\infty} M_0 \exp(-z/\lambda) {\rm d}z \\ &\simeq 1.5(\mu_{\rm B}/{\rm Mn}), \end{aligned} \tag{8}$$

where $M_0 = 2.5\ \mu_{\rm B}$/Mn is the saturation magnetization estimated from the SQUID measurement. This is comparable to the spin magnetic moment estimated from the present XMCD experiments (1.2-1.3 $\mu_{\rm B}$/Mn). The remaining difference between $M_{\rm av}$ and the experimental value may be attributed to the systematic errors due to the uncertainty of the sample volume in the SQUID measurement and the uncertainty of the XMCD spin sum rule [8]. Indeed, it has been pointed out that the application of the XMCD spin sum rule to early transition metals such as Mn may results in errors [14], especially for $Mn^{3+}$ ($3d^4$) systems [15]. The non-negligible spin-orbit coupling for the $Mn^{3+}$ ion may also lead to the inaccuracy of the XMCD sum rule, which may also account for the difference between $M_{\rm av}$ and the experimental magnetic moment.

Supplementary Fig. 4 shows the temperature ($T$) dependence of the resistivity ($\rho$) for the LSMO/STO, partially relaxed LSMO/LAO, and fully strained LSMO/LAO thin films. Since the LSMO/STO film prepared for the XMCD measurement is grown on a conductive Nb-doped STO substrate, resistivity measurements are not feasible. Therefore, we show here the resistivity data for another LSMO thin film grown on a non-doped STO substrate, which was grown essentially under the same conditions as the film studied by XMCD [1]. These $\rho$-$T$ curves clearly shows that the LSMO/STO and partially relaxed LSMO/LAO thin films are in the metallic phase at the temperature where XMCD was measured (270 K for LSMO/STO and 30 K for LSMO/LAO), while the fully strained LSMO/LAO film is insulating. The metal-insulator transition temperature ($T_p$) is estimated to be $345 \pm 5$ K for LSMO/STO and $290 \pm 5$ K for partially relaxed LSMO/LAO.

---

**Supplementary References**


[1] K. Horiba *et al.*, Phys. Rev. B **71**, 155420 (2005).

[2] G. van der Laan, R. V. Chopdekar, Y. Suzuki, and E. Arenholz, Phys. Rev. Lett. **105**, 067405 (2010).

[3] J. Stöhr and H. König, Phys. Rev. Lett. **75**, 3748 (1995).

[4] H. A. Dürr and G. van der Laan, Phys. Rev. B **54**, R760 (1996).

[5] G. van der Laan, J. Phys. Condens. Matter **10**, 3239 (1998).

[6] G. van der Laan, Phys. Rev. B **57**, 5250 (1998).

[7] B. T. Thole, P. Carra, F. Sette, and G. van der Laan, Phys. Rev. Lett. **68**, 1943 (1992).

[8] P. Carra, B. T. Thole, M. Altarelli, and X. Wang, Phys. Rev. Lett. **70**, 694 (1993).

[9] Y. Konishi *et al.*, J. Phys. Soc. Jpn. **68**, 3790 (1999).

[10] F. Tsui, M. C. Smoak, T. K. Nath, and C. B. Eom, Appl. Phys. Lett. **76**, 2421 (2000).

[11] C. Kwon *et al.*, J. Magn. Magn. Mater. **172**, 229 (1997).

[12] K. Yoshimatsu *et al.*, Appl. Phys. Lett. **94**, 071901 (2009).

[13] R. Nakajima, J. Stöhr, and Y. U. Idzerda, Phys. Rev. B **59**, 6421 (1999).

[14] Y. Teramura, A. Tanaka, and T. Jo, J. Phys. Soc. Jpn. **65**, 1053 (1996).

[15] C. Piamonteze, P. Miedema, and F. M. F. de Groot, J. Phys. Conf. Ser. **190**, 012015 (2009).
